# Supplementary material for: SS-DC: Spatial-Spectral Decoupling and Coupling Across Visible-Infrared Gap for Domain Adaptive Object Detection
Source: arXiv:2507.12017 source file (2025-07-16)
Supplement: Supplementary file 1 [file 4_Appendix.tex]

\section{Appendex}
\subsection{The efficientness of new experiment protocol}

\subsection{The difference between our method and previous methods}

\subsection{Code of method}

\subsection{The difference between three modes}

\subsection{Expriment settings}
